# Supplementary material for: Spontaneous Hall effect induced by strain in Pr$_2$Ir$_2$O$_7$ epitaxial thin films
Source: arXiv:1711.07813 source file (2017-11-21)
Supplement: Supplementary file 1 [file Manuscript_Pr2Ir2O7_SM.pdf]

# Supplemental Material for "Spontaneous Hall effect induced by strain in $Pr_2Ir_2O_7$ epitaxial thin films"

Takumi Ohtsuki,[1,*] Zhaoming Tian,[1] Akira Endo,[1] Mario Halim,[1] Shingo Katsumoto,[1] Yoshimitsu Kohama,[1] Koichi Kindo,[1] Satoru Nakatsuji,[1,2] and Mikk Lippmaa[1]

[1]*Institute for Solid State Physics, The University of Tokyo, Kashiwa, Chiba 277-8581, Japan*

[2]*CREST, Japan Science and Technology Agency (JST), 4-1-8 Honcho Kawaguchi, Saitama 332-0012, Japan*

(Dated: November 21, 2017)

* Author to whom correspondence should be addressed. E-mail: ohtsuki@issp.u-tokyo.ac.jp

## Additional characterization by x-ray diffraction

To verify the epitaxial growth of $Pr_2Ir_2O_7$ thin films on YSZ(111), x-ray diffraction (XRD) azimuthal scans of asymmetric reflections were carried out. In Fig. S1(a), scans of the $Pr_2Ir_2O_7$ (662) and the YSZ (331) peaks have the same positions showing three-fold symmetry. In-plane rotated domains are absent in the film, indicating that the $Pr_2Ir_2O_7$ thin films were epitaxially grown on YSZ(111).

A reciprocal space map recorded in the vicinity of the YSZ (331) reflection is shown in Fig. S1(b). The (662) peak of the $Pr_2Ir_2O_7$ thin film is located close to the bulk position marked by an open circle, indicating that the film is relaxed. However, a weak shoulder is visible right under the YSZ (331) peak as shown by the cross-section profile in Fig. S1(c). This clearly shows that there exist some parts in the film where the film lattice is epitaxially locked to the YSZ substrate. The existence of strained grains in the film was verified by scanning transmission electron microscopy (STEM) as shown in Fig. 1 in the main text.

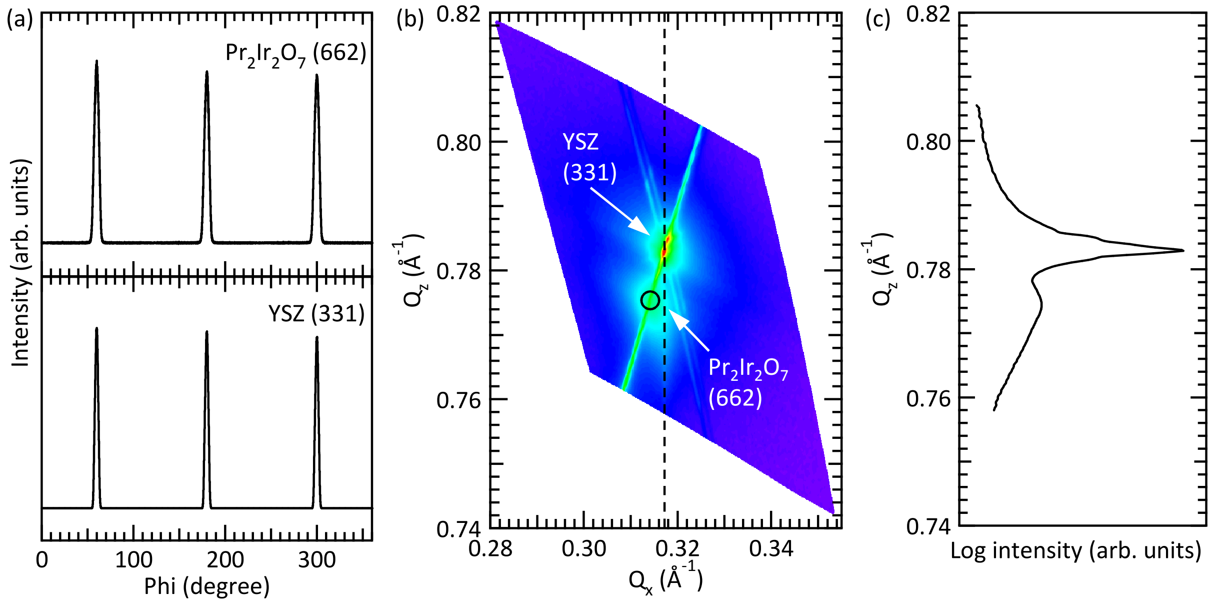


FIG. S1. (a) XRD azimuthal scan of the $Pr_2Ir_2O_7$ (662) (top) and YSZ (331) (bottom) reflections. (b) Reciprocal space map in the vicinity of the YSZ (331) reflection. The upper and lower peaks corresponds to the YSZ (331) and $Pr_2Ir_2O_7$ (662) reflections, respectively. The position at which bulk $Pr_2Ir_2O_7$ appears is marked by open circle (◯). (c) Line profile along the vertical dashed line in (b).

**Estimation of carrier density and Fermi energy**

In this section, carrier density ($n$) and Fermi energy ($E_F$) of $Pr_2Ir_2O_7$ thin film are estimated. For magnetic conductors, Hall resistivity ($\rho_{xy}$) is expressed by the sum of the ordinary Hall term proportional to the magnetic field ($B$) due to the Lorentz force and the anomalous Hall term proportional to the magnetization ($M$) caused by the spin-orbit interaction. This is empirically formulated as $\rho_{xy}(B) = R_0 B + R_s M(B)$, where $R_0$ and $R_s$ is ordinary and anomalous Hall coefficient, respectively. When both sides of this equation are divided by $B$, it is deformed into $\rho_{xy}(B)/B = R_0 + R_s M(B)/B$. Then, $R_0$ is obtained by fitting $\rho_{xy}(B)/B$ with a straight line as a function of $M(B)/B$, and $n$ can be calculated using the relation $R_0 = -1/ne$. Here, $e$ is elementary charge, and $R_0$ is a negative quantity with respect to free electron as $e$ is positive by definition.

In Fig. S2, the plot of $\rho_{xy}(B)/B$ versus $M(B)/B$ and the fitting result are shown. For $\rho_{xy}(B)$ and $M(B)$, experimental data measured at 2 K are used. In the analysis, it is difficult to fit the high $M(B)/B$ region, which corresponds to the low magnetic field region. This deviation from the linear relation indicates that the topological Hall effect generated by the spin chirality [S1] is dominant in the low field region as discussed in the main text. Then, by fitting the low $M(B)/B$ region, $R_0$ is obtained as 3.56 $\mu\Omega$cm/T, and $n$ is calculated as $1.75\times10^{20}$ cm$^{-3}$. This low carrier density is similar to the value reported for the stoichiometric bulk samples [S2].

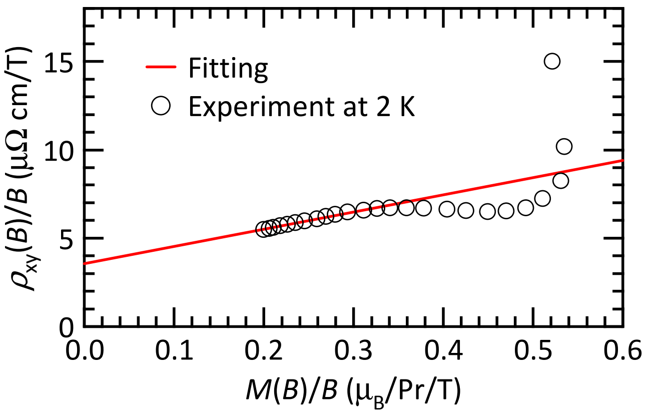


FIG. S2. Plot of $\rho_{xy}(B)/B$ versus $M(B)/B$. For the plot (open circle (◯)), experimentally obtained $\rho_{xy}(B)$ and $M(B)$ measured at 2 K are used, which are shown in Figs. S3(l) and S4, respectively. Red line represents the fitting result with a linear function.

Next, the Fermi wavenumber $k_F$ is obtained as 0.173 $Å^{-1}$ by substituting $n$ in the relation $k_F = (3\pi^2 n)^{1/3}$ for the free electron gas. In addition, $E_F$ is expressed as $E_F = \hbar^2 k_F^2/2m^*$ assuming the parabolic dispersion in the quadratic band touching system. Here, $\hbar$ is Dirac's constant, and $m^*$ is the effective mass that is reported to be $6.3m_0$ ($m_0$ is free electron mass) from the band dispersion observed by angle-resolved photoelectron emission spectroscopy [S3]. As a result, $E_F$ is estimated to be ∼18 meV, which is consistent with the value obtained by an optical measurements [S4].

**Hall measurement at temperatures above 2 K**

Hall resistivity ($\rho_{xy}$) of the $Pr_2Ir_2O_7$ thin film is plotted as a function of the magnetic field ($B$) in Fig. S3. Data obtained at various temperatures above 2 K are displayed. As mentioned in the main text, under 50 K, $\rho_{xy}(B)$ draws a hysteresis loop around zero field, and has a non-zero spontaneous value even at zero field. This non-zero spontaneous Hall resistivity gradually grows toward 2 K. The hysteresis disappears above 50 K, resulting in zero remnant value.

**Magnetization curve**

Figure S4 shows the magnetic field dependence of the magnetization ($M(B)$) of the $Pr_2Ir_2O_7$ thin film measured at 2 K. No hysteresis is observed. The saturation value ∼1 $\mu_B$ is consistent with the Ising spin anisotropy of the Pr $4f$ moments and with the bulk case [S1].

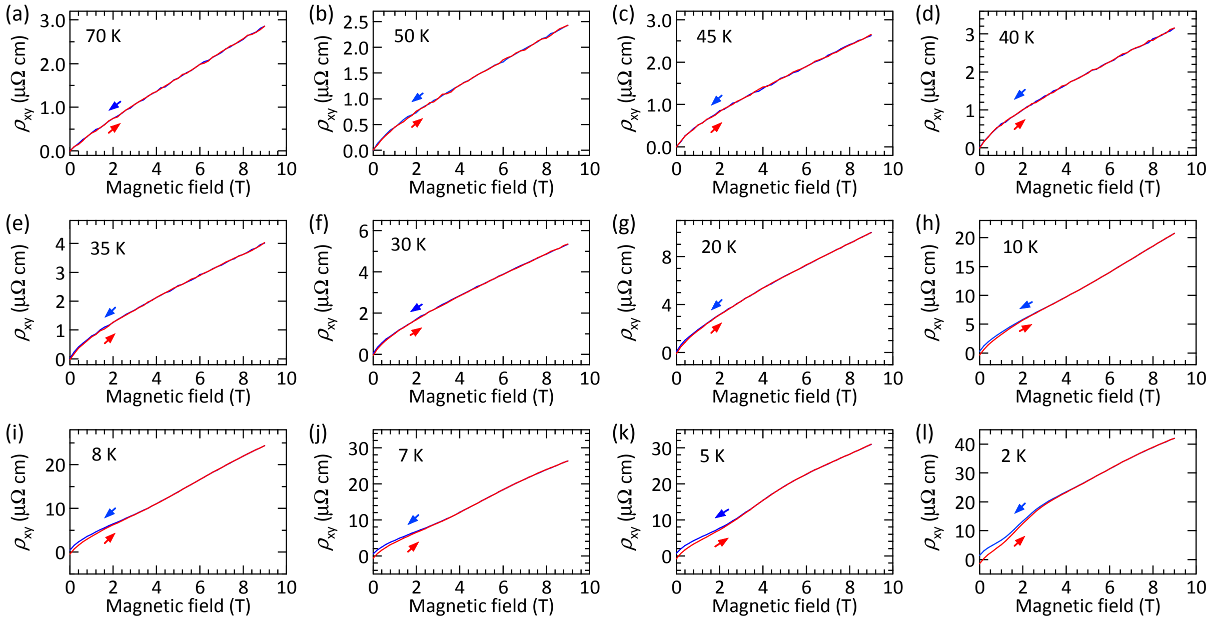


FIG. S3. Hall resistivity ($\rho_{\rm xy}$) of a $Pr_2Ir_2O_7$ thin film as a function of magnetic field ($B$) measured at various temperatures above 2 K. $\rho_{\rm xy}(B)$ is obtained by the equation $[\rho_{\rm xy}(B) - \rho_{\rm xy}(-B)]/2$ to eliminate the $\rho_{\rm xx}$ component. Magnetic field is applied along the [111] direction. Red and blue lines represent up and down sweeps of the magnetic field, respectively.

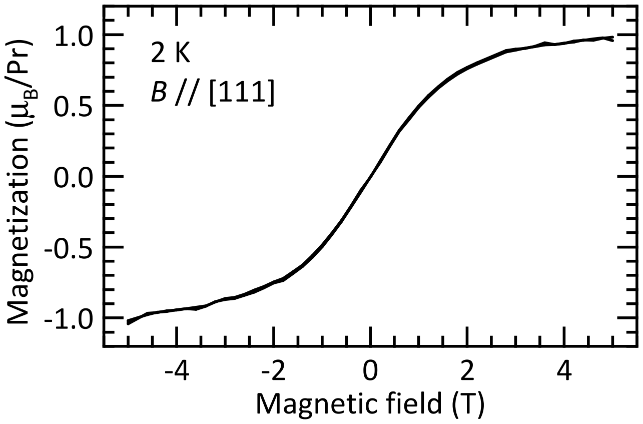


FIG. S4. Magnetization curve of $Pr_2Ir_2O_7$ thin film measured at 2 K. Diamagnetic response from the YSZ substrate is subtracted. Magnetic field is applied along the [111] direction.

## Magnetoresistivity curves at temperatures above 2 K

Figure S5 shows transverse magnetoresistance (MR) ratio curves of the $Pr_2Ir_2O_7$ thin film as a function of the magnetic field $B$, measured at temperatures above 2 K. The MR curve shape is strongly affected by temperature. At temperatures higher than 50 K (Figs. S5(a) and S5(b)), the $Pr_2Ir_2O_7$ thin film shows positive MR as can be seen for conventional metals. On the other hand, negative MR starts to evolve below 50 K (Figs. S5(c)–S5(g)). Interestingly, the onset temperature of negative MR seems to coincide with the temperature at which $\rho_{xx}(0\ \mathrm{T})$ passes through the minimum (Fig. 2(a) in the main text). Furthermore, below 10 K, as the magnetic field is increased (Figs. S5(h)–S5(l)), MR curves minimize at a certain field, above which resistivity increases monotonically. As mentioned in the main text, this upturn in the MR curves originates from a metamagnetic transition [S1]. In this temperature range, it is more obvious that the magnetic field at which the metamagnetic transition occurs becomes lower as the sample is further cooled.

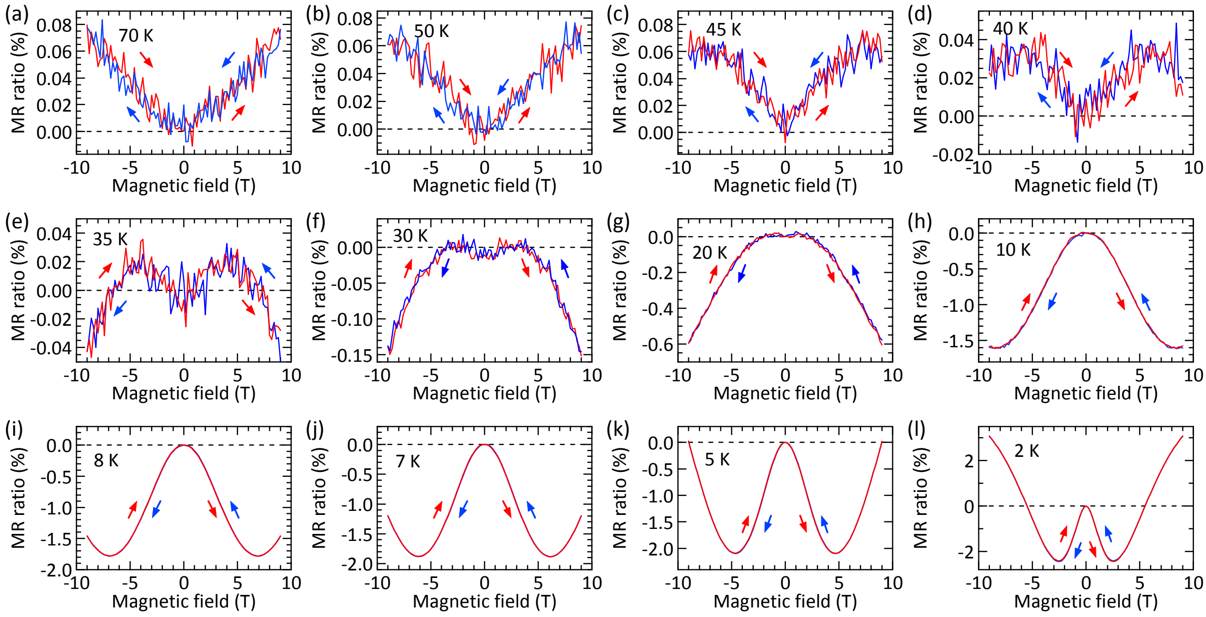


FIG. S5. Transverse MR curves of the $Pr_2Ir_2O_7$ thin film as a function of magnetic field $B$ measured at various temperatures above 2 K. The vertical axes are converted to MR ratio by the equation $[\rho_{xx}(B) - \rho_{xx}(0)]/\rho_{xx}(0) \times 100$. For clarity, dashed lines are drawn at zero percent. Magnetic field is applied along the [111] direction. Red and blue lines correspond to up and down sweeps of the magnetic field, respectively.

**Linear relation between temperature and magnetic field at the minimum observed in the magnetoresistivity curves**

As seen in Fig. 3 in the main text and Supplemental Fig. S5, MR curves of the $Pr_2Ir_2O_7$ thin film show a minimum at a certain magnetic field that is temperature dependent. The relationship between temperature and the magnetic field strength at the MR minimum is summarized in Fig. 4 in the main text, representing the crossover from the 2-in–2-out or the paramagnetic state to the field-polarized 3(1)-in–1(3)-out spin configuration. The data points are replotted on a linear scale in Fig. S6. A linear relationship between temperature and the magnetic field strength is clearly seen.

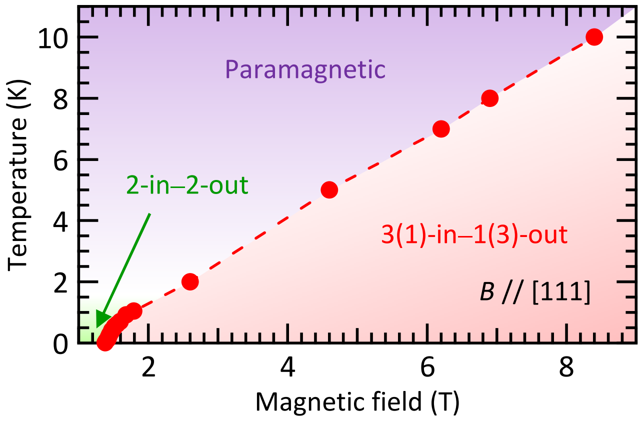


FIG. S6. Linear scale plot of temperature dependence of the crossover-magnetic field where MR curves of $Pr_2Ir_2O_7$ thin film pass through the minimum. Data points are extracted from Fig. 4 in the main text, in which they delineate the crossover from 2-in–2-out to 3(1)-in–1(3)-out spin configuration shown as the right red border. The same plot in semi-logarithmic scale is shown in Fig. 4 in the main text.

## Supplemental References

[S1] Y. Machida, S. Nakatsuji, S. Onoda, T. Tayama, and T. Sakakibara, *Time-reversal symmetry breaking and spontaneous Hall effect without magnetic dipole order*, Nature **463**, 210 (2010).

[S2] S. Nakatsuji, Y. Machida, Y. Maeno, T. Tayama, T. Sakakibara, J. van Duijn, L. Balicas, J. N. Millican, R. T. Macaluso, and Julia Y. Chan, *Metallic spin-liquid behavior of the geometrically*

*frustrated Kondo lattice $Pr_2Ir_2O_7$*, Phys. Rev. Lett. **96**, 087204 (2006).

[S3] T. Kondo, M. Nakayama, R. Chen, J. J. Ishikawa, E.-G. Moon, T. Yamamoto, Y. Ota, W. Malaeb, H. Kanai, Y. Nakashima, Y. Ishida, R. Yoshida, H. Yamamoto, M. Matsunami, S. Kimura, N. Inami, K. Ono, H. Kumigashira, S. Nakatsuji, L. Balents, and S. Shin, *Quadratic Fermi node in a 3D strongly correlated semimetal*, Nat. Commun. **6**, 10042 (2015).

[S4] B. Cheng, T. Ohtsuki, D. Chaudhuri, S. Nakatsuji, M. Lippmaa, and N. P. Armitage, *Dielectric anomalies and interactions in the three-dimentional quadratic band touching Luttinger semimetal $Pr_2Ir_2O_7$*, (unpublished).
